# Supplementary material for: Sequential Quadratic Optimization for Stochastic Optimization with Deterministic Nonlinear Inequality and Equality Constraints
Source: arXiv:2302.14790 source file (2023-02-28)
Supplement: Supplementary file 1 [file appendix.tex]

\section{Deterministic Setting}

The next lemma shows the sequence of $\{\alpha_k^{\min}\}$ is bounded away from zero if $\{\tau_k\}$ is bounded away from zero.
\blemma\label{lem.stepsize_lb}
Suppose $\beta_{\min}\in\R{}_{>0}$ is a lower bound of the sequence $\{\beta_k\}\subset\R{}_{>0}$. If there exists a constant $\tau_{\min}\in\R{}_{>0}$ such that $\tau_k = \tau_{\min}$ for all sufficiently large $k\in\N{}$, then the sequence of $\{\alpha_k^{\min}\}$ is bounded away from zero.
\elemma
\bproof
By \eqref{eq.alpha_min} and Corollary~\ref{cor.stoch_perf} (d), we know that if such a constant $\tau_{\min}\in\R{}_{>0}$ exists, it follows that for all $k\in\N{}$,
\bequationNN
\alpha_k^{\min} = \tfrac{2(1-\eta)\beta_k\xi_k\tau_k}{\tau_kL+\Gamma} \geq \tfrac{2(1-\eta)\beta_{\min}\xi_{\min}\tau_{\min}}{\tau_{\min}L+\Gamma} > 0.
\eequationNN
Then we conclude the statement
\eproof

Next, we provide an upper bound of merit function decrease.

\blemma\label{lem.suff_decrease_deterministic}
Suppose we run Algorithm~\ref{alg.sqp} with $g_k = \nabla f_k$ for all $k\in\N{}$, then 
\bequation\label{eq.suff_decrease_deterministic}
\phi(x_k+\alphatrue_k\dtrue_k,\tautrue_k) - \phi(x_k,\tautrue_k) \leq -\eta\alphatrue_k\beta_k\Delta l(x_k,\tautrue_k,\nabla f_k,\dtrue_k).
\eequation
\elemma
\bproof
When $\dtrue_k = 0$, \eqref{eq.suff_decrease_deterministic} holds trivially by \eqref{eq.model_reduction}. When $\dtrue_k \neq 0$, by Assumption~\ref{ass.prob}, \eqref{eq.model_reduction}, \eqref{eq.alpha_min}--\eqref{eq.alpha_max}, Corollary~\ref{cor.stoch_perf}, and Lemma~\ref{lem.varphi_nonpositive}, we have that
\bequationNN
\baligned
&\phi(x_k + \alphatrue_k\dtrue_k,\tautrue_k) - \phi(x_k,\tautrue_k) \\
= \ &\tautrue_k(f(x_k + \alphatrue_k\dtrue_k) - f_k) + \|c(x_k + \alphatrue_k\dtrue_k)\|_2 - \|c_k\|_2 \\
\leq \ &\alphatrue_k\tautrue_k\nabla f_k^T\dtrue_k + \|c_k + \alphatrue_kJ_k\dtrue_k\|_2 - \|c_k\|_2 + \tfrac{\tautrue_kL+\Gamma}{2}(\alphatrue_k)^2\|\dtrue_k\|_2^2 \\ 
\leq \ &\alphatrue_k\tautrue_k\nabla f_k^T\dtrue_k + (1-\eta)\alphatrue_k\beta_k\Delta l(x_k,\tautrue_k,\nabla f_k,\dtrue_k) - \alphatrue_k(\|c_k\|_2 - \|c_k + J_k\dtrue_k\|_2) \\
= \ &-\alphatrue_k\Delta l(x_k,\tautrue_k,\nabla f_k,\dtrue_k) + (1-\eta)\alphatrue_k\beta_k\Delta l(x_k,\tautrue_k,\nabla f_k,\dtrue_k) \\
\leq \ &-\eta\alphatrue_k\beta_k\Delta l(x_k,\tautrue_k,\nabla f_k,\dtrue_k),
\ealigned
\eequationNN
which concludes the statement.
\eproof

Now we state the final theorem for the deterministic setting.
\begin{theorem}
Suppose Assumptions~\ref{ass.prob} and~\ref{ass.H} hold. Suppose we choose $\beta_k=\beta$ for all $k\in\N{}$ satisfying \eqref{eq.beta_constraint}. If for all sufficiently large iterations $k\in\N{}$, there always exists a constant $\omega_c\in [0,1)$ such that
\bequation\label{eq.sufficient_progress_constraint_violation}
\|c_k + J_kv_k\|_2 \leq \omega_c\|c_k\|_2,
\eequation
then $\{\tautrue_k\}$ is bounded away from zero and 
\bequation\label{eq.deterministic_result_1}
\left\{\left\|\bbmatrix \nabla f_k + J_k^T\ytrue_k - \lambdatrue_k \\ c_k \\ [x_k]^- \\ [\lambdatrue_k]^- \\ x_k^T\lambdatrue_k \ebmatrix\right\|\right\} \to 0.
\eequation
Otherwise, $\{\|J_kv_k\|\}\to 0$, and if $\{\tautrue_k\}$ is bounded away from zero, then
\bequation\label{eq.deterministic_result_2}
\left\{\left\|\bbmatrix \nabla f_k + J_k^T\ytrue_k - \lambdatrue_k \\ [x_k]^- \\ [\lambdatrue_k]^- \\ x_k^T\lambdatrue_k \ebmatrix\right\|\right\} \to 0.
\eequation
\end{theorem}
\bproof
If \eqref{eq.sufficient_progress_constraint_violation} holds for all sufficiently large iterations, by Corollary~\ref{cor.stoch_perf} (b) and Lemma~\ref{lem.tau_away_from_zero}, we know $\tautrue_k = \tautruemin$ for all sufficiently large $k\in\N{}$. Suppose $\tautrue_{k_{\tau}} = \tautruemin$, then by Assumption~\ref{ass.prob}, and Lemmas~\ref{lem.stepsize_lb}--\ref{lem.suff_decrease_deterministic}, it follows that
\bequation\label{eq.telescoping_1}
\baligned
&-\infty < \phi(x_{k_{\tau}+K},\tautruemin) - \phi(x_{k_{\tau}},\tautruemin) = \sum_{k=k_{\tau}}^{k_{\tau}+K-1}\left(\phi(x_{k+1},\tautruemin) - \phi(x_k,\tautruemin)\right) \\
\leq \ &-\sum_{k=k_{\tau}}^{k_{\tau}+K-1} \eta\alphatrue_k\beta\Delta l(x_k,\tautruemin,\nabla f_k,\dtrue_k) \\
\leq \ &-\tfrac{2\eta(1-\eta)\xi_{\min}\tautruemin\beta^2}{\tautruemin L+\Gamma}\cdot\sum_{k=k_{\tau}}^{k_{\tau}+K-1} \Delta l(x_k,\tautruemin,\nabla f_k,\dtrue_k).
\ealigned
\eequation
Let $K\to\infty$, it follows that $\left\{\Delta l(x_k,\tautrue_k,\nabla f_k,\dtrue_k)\right\}\to 0$. By Assumption~\ref{ass.H}, Corollary~\ref{cor.stoch_perf} (c), and \eqref{eq.sufficient_progress_constraint_violation}, we further have 
\bequationNN
\baligned
\Delta l(x_k,\tautrue_k,\nabla f_k,\dtrue_k) &\geq \min\left\{\zeta\tautruemin,\sigma\right\}\cdot(\|\dtrue_k\|_2^2 + (\|c_k\|_2 - \|c_k + J_k\dtrue_k\|_2)) \\
&\geq \min\left\{\zeta\tautruemin,\sigma\right\}\cdot(\|\dtrue_k\|_2^2 + (1-\omega_c)\cdot\|c_k\|_2),
\ealigned
\eequationNN
which implies that $\{\max\{\|\dtrue_k\|,\|c_k\|\}\}\to 0$. From KKT conditions of \eqref{prob.d}, we know for any $k\in\N{}$, the primal-dual iterate $(\dtrue_k,\ytrue_k,\lambdatrue_k)$ always satisfies
\bequationNN
\left\|\bbmatrix \nabla f_k + H\dtrue_k + J_k^T\ytrue_k - \lambdatrue_k \\ J_k(\dtrue_k - v_k) \\ [x_k + \dtrue_k]^- \\ [\lambdatrue_k]^- \\ (x_k + \dtrue_k)^T\lambdatrue_k \ebmatrix\right\| = 0,
\eequationNN
which implies \eqref{eq.deterministic_result_1} by $\{\max\{\|\dtrue_k\|,\|c_k\|\}\}\to 0$.

When \eqref{eq.sufficient_progress_constraint_violation} is not satisfied for all sufficiently large $k\in\N{}$, if $\{\tautrue_k\}$ is still bounded away from zero, then \eqref{eq.telescoping_1} still holds, which implies $\left\{\Delta l(x_k,\tautrue_k,\nabla f_k,\dtrue_k)\right\}\to 0$. Then by Assumption~\ref{ass.H}, and Corollary~\ref{cor.stoch_perf} (a) and (c), we further have 
\bequationNN
\baligned
\Delta l(x_k,\tautrue_k,\nabla f_k,\dtrue_k) &\geq \min\left\{\zeta\tautruemin,\sigma\right\}\cdot(\|\dtrue_k\|_2^2 + (\|c_k\|_2 - \|c_k + J_k\dtrue_k\|_2)) \\
&= \min\left\{\zeta\tautruemin,\sigma\right\}\cdot(\|\dtrue_k\|_2^2 + (\|c_k\|_2 - \|c_k + J_kv_k\|_2)) \\
&\geq \min\left\{\zeta\tautruemin,\sigma\right\}\cdot\|\dtrue_k\|_2^2,
\ealigned
\eequationNN
which implies that $\{\|\dtrue_k\|\}\to 0$. From $\{\|\dtrue_k\|\}\to 0$, we further have $\{\|v_k\|\}\to 0$ and $\{\|J_kv_k\|\}\to 0$. From KKT conditions of \eqref{prob.d} and using the same logic as the previous case, we know \eqref{eq.deterministic_result_2} holds.

If $\{\tautrue_k\}\to 0$ \bz{and we choose step sizes $\alphatrue_k := \min\left\{1,\tfrac{2(1-\eta)\Delta l(x_k,\tautrue_k,\nabla f_k,\dtrue_k)}{(\tautrue_k L +\Gamma)\|\dtrue_k\|_2^2}\right\}$}, then by Assumptions~\ref{ass.prob} and~\ref{ass.H} Corollary~\ref{cor.stoch_perf} (c) and \eqref{eq.wk_2_lb}, we have
\bequationNN
\baligned
\alphatrue_k &\geq \min\left\{1,\tfrac{2(1-\eta)(\tautrue_k\zeta\|\dtrue_k\|_2^2 + \sigma(\|c_k\|_2 - \|c_k + J_k\dtrue_k\|_2))}{(\tau_{-1}L+\Gamma)\|\dtrue_2\|_2^2}\right\} \\
&\geq \min\left\{1,\tfrac{2(1-\eta)\sigma(\|c_k\|_2 - \|c_k + J_k\dtrue_k\|_2)}{(\tau_{-1}L+\Gamma)\|\dtrue_2\|_2^2}\right\} \\
&= \min\left\{1,\tfrac{2(1-\eta)\sigma(\|c_k\|_2 - \|c_k + J_kJ_k^Tw_k\|_2)}{(\tau_{-1}L+\Gamma)\|\dtrue_2\|_2^2}\right\} \\
&\geq \min\left\{1,\tfrac{(1-\eta)\sigma/\kappa_c\cdot(\lambda_{\inf}\|J_k^Tw_k\|_2^2 + 2\mu_k\|v_k^u\|_2^2)}{(\tau_{-1}L+\Gamma)\|\dtrue_2\|_2^2}\right\} \\
&\geq \min\left\{1,\tfrac{(1-\eta)\sigma\cdot\min\{\lambda_{\inf},2\mu_k\}}{\kappa_c(\tau_{-1}L+\Gamma)}\right\}.
\ealigned
\eequationNN
By Assumption~\ref{ass.prob}, and Lemmas~\ref{lem.stepsize_lb}--\ref{lem.suff_decrease_deterministic}, it follows that
\bequationNN
\baligned
&-\infty < \phi(x_{k_{\tau}+K},\tautruemin) - \phi(x_{k_{\tau}},\tautruemin) = \sum_{k=k_{\tau}}^{k_{\tau}+K-1}\left(\phi(x_{k+1},\tautruemin) - \phi(x_k,\tautruemin)\right) \\
\leq \ &-\sum_{k=k_{\tau}}^{k_{\tau}+K-1} \eta\alphatrue_k\beta\Delta l(x_k,\tautruemin,\nabla f_k,\dtrue_k) \\
\leq \ &-\beta\eta\cdot\min\left\{1,\tfrac{(1-\eta)\sigma\cdot\min\{\lambda_{\inf},2\mu_k\}}{\kappa_c(\tau_{-1}L+\Gamma)}\right\}\cdot\sum_{k=k_{\tau}}^{k_{\tau}+K-1} \Delta l(x_k,\tautruemin,\nabla f_k,\dtrue_k).
\ealigned
\eequationNN
Let $K\to\infty$, it follows that $\left\{\Delta l(x_k,\tautrue_k,\nabla f_k,\dtrue_k)\right\}\to 0$. By Assumption~\ref{ass.H}, Corollary~\ref{cor.stoch_perf} (c), and Lemma~\ref{lem.wk_2_lb}, we further have 
\bequationNN
\baligned
\Delta l(x_k,\tautrue_k,\nabla f_k,\dtrue_k) &\geq \tautrue_k\zeta\|\dtrue_k\|_2^2 + \sigma(\|c_k\|_2 - \|c_k + J_k\dtrue_k\|_2) \\
&\geq \sigma(\|c_k\|_2 - \|c_k + J_k\dtrue_k\|_2) \\
&\geq \sigma\kappa_{w,2}\|w_k\|_2^2,
\ealigned
\eequationNN
which further implies that $\{\|w_k\|\}\to 0$ and $\{\|J_kv_k\|\}\to 0$.
\eproof
